# Supplementary material for: Large Investment Model
Source: arXiv:2408.10255 source file (2024-08-22)
Supplement: Supplementary file 1 [file appendix1.tex]

\clearpage
\section{Appendix: Numerical Experiment}\label{sec_experiment}
\subsection{Experiment Setup}
We collect the 1-min candlestick data of all 5226 stocks in China A-share market and of 9 futures (including 7 commodity futures: RU, PB, B, SP, P, FB, PP and for 2 stock index futures IF and IH). These stocks and futures belong to Shanghai Stock Exchange (SSE), Shenzhen Stock Exchange (SZSE), Shanghai Futures Exchange (SHFE), Dalian Commodity Exchange (DCE) and China Financial Futures Exchange (CFFEX). Please refer to Table~\ref{tab:stock-futures} for details.

To enhance computational efficiency, we opted not to employ rolling training, a method commonly used in real-world strategy research. Rolling training, while effective for dynamically updating models, can be computationally intensive due to the constant re-training required as new data becomes available. Instead, we chose to define fixed time periods for the training, validation, and test sets, respectively. This approach allows for a more streamlined and less resource-intensive process while still providing robust evaluation metrics. For time-series prediction, we utilized a standard moving window approach. Specifically, we set the context window size to 120 minutes, which determines the historical data length used to predict future values, and the horizon window size to 30 minutes, which defines the prediction target. These window sizes are chosen to balance the trade-off between capturing sufficient historical information and maintaining timely predictions. In terms of input features, we selected a range of basic data features that are fundamental to financial modeling. These features include close prices, trading volume, and volume-weighted average price (VWAP), calculated at both 1-minute and 5-minute granularities. The choice of these granularities ensures that the model can capture both short-term and slightly longer-term market dynamics, which are crucial for accurate predictions in high-frequency trading environments.

For each financial instrument, we divided the data into training, validation, and test sets based on the following predefined periods:
\begin{itemize}[noitemsep,topsep=0pt]
    \item \textbf{Training set:} 2017-01-03 to 2021-04-27.
    \item \textbf{Validation set:} 2021-04-27 to 2022-04-27.
    \item \textbf{Test set:} 2022-04-27 to 2023-04-27.
\end{itemize}
This structured division of datasets allows for a thorough evaluation of the model’s performance across different market conditions. The training period was chosen to include a diverse range of market environments, ensuring the model learns from varied conditions. The validation period serves to fine-tune model parameters and prevent overfitting, while the test period provides an unbiased evaluation of the model’s predictive power in an out-of-sample scenario. By carefully selecting these periods, we ensure that the model's performance is robust and generalizes well to new data, thereby enhancing its practical applicability in real-world trading strategies.

We conducted a series of experiments to rigorously evaluate the performance of two distinct paradigms in quantitative modeling. In Experiment 1, we implemented a two-stage approach where we first pre-trained a foundation model using a comprehensive dataset that included both stock and futures data. This initial training phase allowed the model to capture broad, cross-instrument patterns and correlations present in the entire dataset. After the pre-training phase, the foundation model was fine-tuned for each specific futures instrument, utilizing data exclusively related to that particular instrument. This fine-tuning process was designed to adapt the model to the unique characteristics and idiosyncrasies of each futures market, thereby enhancing its predictive accuracy when applied to the test set. In contrast, Experiment 2 served as a benchmark by employing a more traditional approach. Here, we trained individual models directly on the data for each futures instrument, without the benefit of a pre-trained foundation model. These models, each tailored to a specific instrument from the outset, were then used to make predictions on the same test set. By comparing the results from these two paradigms, we aimed to assess the potential benefits of a foundation model in terms of both predictive performance and the ability to generalize across different financial instruments. This comparative analysis provides valuable insights into the effectiveness of pre-training on diverse financial datasets and the subsequent fine-tuning for instrument-specific predictions.

The effectiveness of these two approaches was compared through a backtesting process by applying them to historical market data on test set period, providing insights into the relative strengths and weaknesses of each technical route. This technique allows traders and researchers to simulate how a strategy would have performed in the past, providing insights into its potential future performance. By analyzing the historical returns, risks, and drawdowns of a strategy, backtesting helps in identifying strengths and weaknesses, refining strategy parameters, and improving decision-making. It also enables the detection of overfitting and helps ensure that the strategy is robust and reliable across different market conditions. Ultimately, backtesting serves as a critical step in the development and validation of quantitative trading strategies before they are deployed in live trading environments.

\begin{table}[ht]
    \centering
    \begin{tabular}{c|c|c}
    \hline
         Name & Code & Exchange\\
         \hline
        2037 Stocks & -- & SSE\\
        2578 Stocks & -- & SZSE\\
         Rubber Futures & RU & SHFE\\
         Lead Futures & PB & SHFE\\
         Soybean No. 2 Futures& B & DCE\\
         Hot Rolled Steel Coil Futures & SP & SHFE\\
         Palm Oil Futures & P & DCE\\
         Fiberboard Futures & FB & DCE\\
         Polypropylene Futures & PP & DCE\\
        CSI 300 Index Futures & IF & CFFEX\\
        SSE 50 Index Futures & IH & CFFEX\\
        \hline
    \end{tabular}
    \caption{The instruments and their exchanges used in experiment.}
    \label{tab:stock-futures}
\end{table}

\subsection{Evaluation Criteria for Back-Testing}
In quantitative investment, back-testing is a critical process used to evaluate the performance of a trading strategy using historical data. When coding for backtesting a quantitative investment strategy, it is crucial to ensure that the implementation accurately reflects the strategy’s logic while maintaining computational efficiency. The first step is to organize historical price data \( \{P_t\} \) into a structured time series, where \( P_t \) denotes the asset price at time \( t \). The strategy's trading signals \( S_t \in \{-1, 0, 1\} \), representing sell, hold, and buy actions, respectively, are generated based on the strategy’s rules. Portfolio returns \( R_t \) are then computed as \( R_t = S_{t-1} \cdot \frac{P_t - P_{t-1}}{P_{t-1}} \). To simulate transaction costs accurately, we define a cost function \( C_t = \kappa \cdot |S_t - S_{t-1}| \cdot P_t \), where \( \kappa \) represents the transaction cost rate (e.g., a percentage of the traded value). The adjusted return accounting for transaction costs is given by \( R_t^{\text{net}} = R_t - C_t \). Efficient backtesting code should leverage vectorized operations to process large datasets, reducing the need for iterative loops, and should utilize high-performance libraries such as NumPy or pandas for array manipulations. By incorporating accurate transaction cost simulations and optimizing the code structure, the backtest can provide a realistic and computationally efficient evaluation of the strategy's performance.

Several key evaluation criteria are commonly used to assess the effectiveness and robustness of a strategy. This section introduces four essential metrics: Information Coefficient (IC), Annual Return, Maximal Drawdown, and Sharpe Ratio. Each criterion offers unique insights into different aspects of the strategy's performance.

\begin{itemize}[noitemsep,topsep=0pt] 
\item \underline{Information Coefficient (IC)}: Information Coefficient is a measure of the correlation between the predicted returns and the actual returns of a portfolio. It is often used to evaluate the predictive power of a model or strategy. The formula is defined as:
\[
IC = \frac{\text{Cov}(R_p, \hat{R_p})}{\sigma_{R_p} \sigma_{\hat{R_p}}}
\]
Where:
\begin{itemize}
    \item \(R_p\) is the actual return of the portfolio.
    \item \(\hat{R_p}\) is the predicted return.
    \item \(\sigma_{R_p}\) and \(\sigma_{\hat{R_p}}\) are the standard deviations of the actual and predicted returns, respectively.
    \item \(\text{Cov}(R_p, \hat{R_p})\) is the covariance between the actual and predicted returns.
\end{itemize}
The Information Coefficient quantifies the strength of the relationship between predicted and actual returns. A higher IC indicates better predictive accuracy of the strategy, which implies more reliable forecasts and potential for better performance.

\item \underline{Annual Return}: Annual Return refers to the compounded return that a strategy or portfolio generates over a year. It is a straightforward measure of the average performance over time.
\[
AR = \left( \prod_{t=1}^{T} (1 + r_t) \right)^{\frac{1}{T}} - 1
\]
Where:
\begin{itemize}
    \item \(r_t\) is the return in each period \(t\).
    \item \(T\) is the total number of periods.
\end{itemize}
The Annual Return metric provides an estimate of the strategy's average yearly growth rate, allowing investors to gauge the long-term profitability of the strategy.

\item \underline{Maximal Drawdown}: Maximal Drawdown (MDD) measures the largest peak-to-trough decline in the value of a portfolio over a given period. It is an indicator of downside risk.
\[
MDD = \min \left( \frac{V_t - V_{\text{peak}}}{V_{\text{peak}}} \right)
\]
Where:
\begin{itemize}
    \item \(V_t\) is the portfolio value at time \(t\).
    \item \(V_{\text{peak}}\) is the highest portfolio value observed up to time \(t\).
\end{itemize}
Maximal Drawdown highlights the worst-case scenario in terms of losses from a peak value, providing a measure of the potential risk of significant declines in portfolio value.

\item \underline{Sharpe Ratio}: The Sharpe Ratio is a widely used measure of risk-adjusted return. It is calculated as the ratio of the excess return of the portfolio (over the risk-free rate) to the standard deviation of those returns.
\[
SR = \frac{R_p - R_f}{\sigma_p}
\]
Where:
\begin{itemize}
    \item \(R_p\) is the portfolio return.
    \item \(R_f\) is the risk-free rate.
    \item \(\sigma_p\) is the standard deviation of the portfolio's returns.
\end{itemize}
The Sharpe Ratio evaluates how well the return of a strategy compensates for the risk taken. A higher Sharpe Ratio indicates that the strategy is generating higher returns per unit of risk, making it a crucial metric for comparing different strategies.
\end{itemize} 
These evaluation criteria, when used together, provide a comprehensive view of a strategy's performance, balancing risk and return to determine its potential viability in real-world applications.

\subsection{Result and Analysis}
\begin{table*}

    \centering
    \begin{tabular}{c|cc|cc|cc|cc}
    \hline
       \multirow{2}{*}{Futures}  & \multicolumn{2}{c|}{Annual Return}  &  \multicolumn{2}{c|}{Sharpe Ratio}  &  \multicolumn{2}{c|}{Maximal Drawdown}  &  \multicolumn{2}{c}{IC} \\
    \cline{2-9}
     & Universal & Task-specific	& Universal &	Task-specific	& Universal &	Task-specific	& Universal & Task-specific\\
    \hline
RU & 1.231 & 1.0199	& 2.499	& 0.184 & 0.00769 &	0.04152	& 0.13257 & 0.07825\\
PB & 1.129 & 1.0578	& 2.56 &	1.51	& 0.00744 &	0.00534	& 0.13837 &	0.09013\\
B  & 1.061 & 1.0108	& 2.21	& 0.281	& 0.00409 &	0.02020	& 0.08292 &	0.07815\\
SP & 1.104 & 1.0555	& 2.16	& 0.311	& 0.00763 &	0.13417	& 0.10838 &	0.06431\\
P  & 1.131 & 1.327	& 2.07	& 0.974	& 0.01144 &	0.10845	& 0.05044 &	0.0508\\
FB	&1.111 	&1.1123	& 2.00	& 0.785	& 0.00524 &	0.08270	& 0.14184 &	0.10714\\
PP	&1.130 	&1.0478	& 1.62	& 0.64	& 0.01416 &	0.03671	& 0.10069 &	0.03479\\
IF	&1.098 	&0.99968 & 1.27	& 0.0027	& 0.01189 &	0.02391	& 0.06021 &	0.01210\\
IH	& 1.065 &	1.0794	& 1.26	& 0.885	& 0.00832 &	0.03282	& 0.07285 &	0.0465\\
    \hline
    \end{tabular}
    \caption{Comparison of the universal modeling used in LIM and task-specific modeling used in traditional quantitative investment research. We list the results according to criteria annual return, Sharpe ratio, maximal drawdown and IC. The experiment results including 7 commodity futures RU, PB, B, SP, P, FB, PP and 2 stock index futures IF and IH.}
    \label{tab:comparison_stocks_futures}
\end{table*}

\begin{figure*}
	\centering
		\includegraphics[scale=0.4]{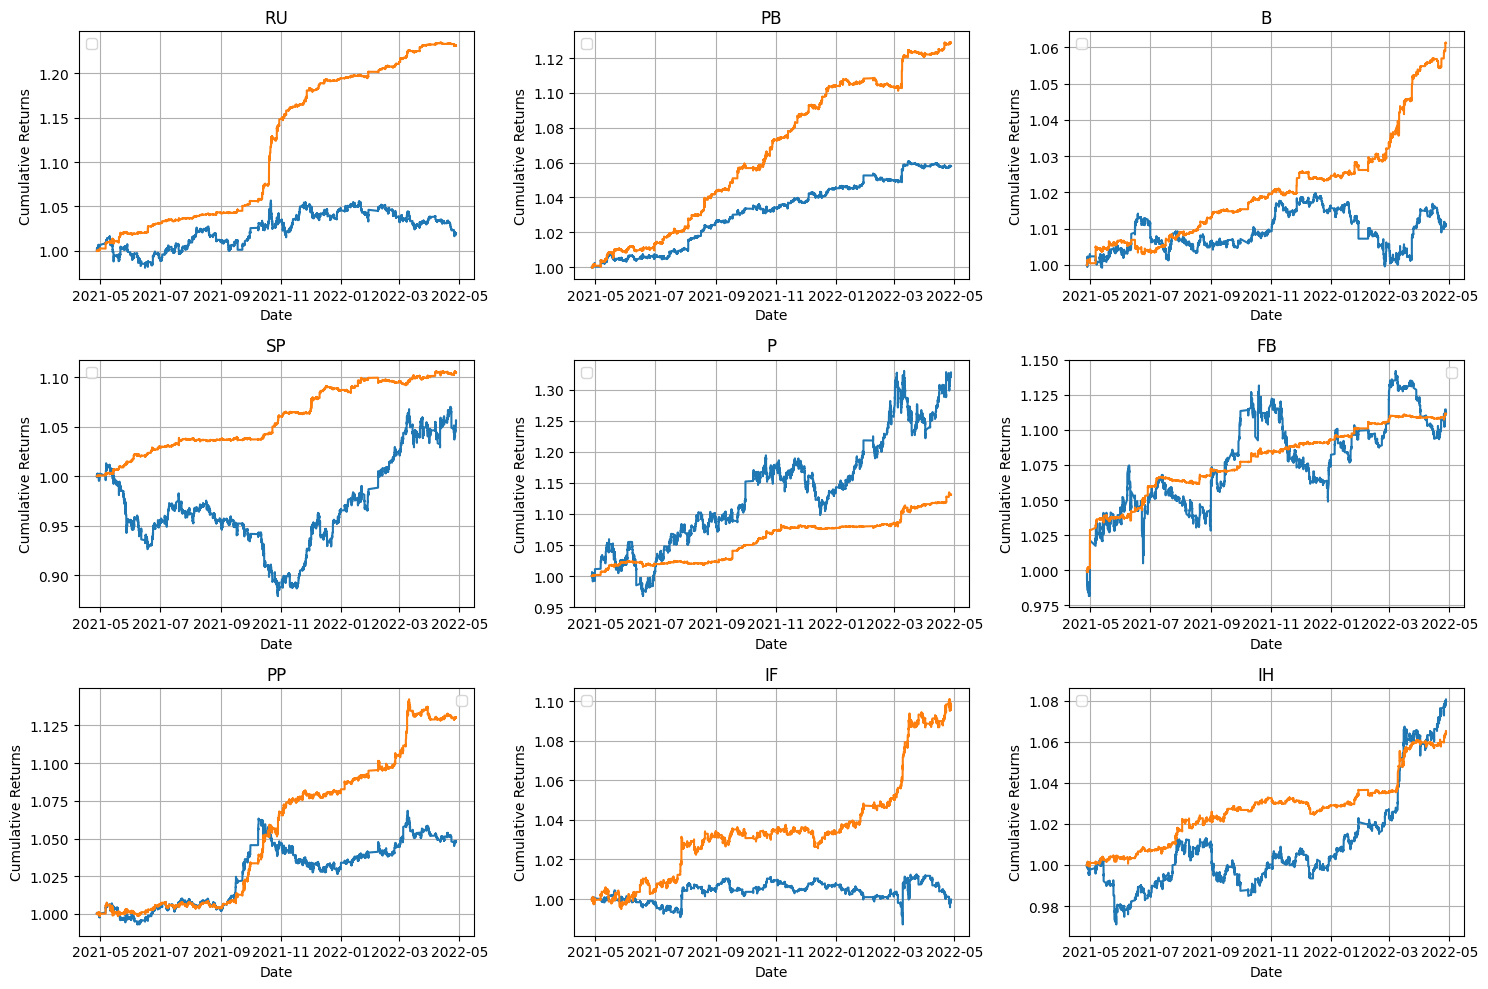}
	\caption{Comparison of the netvalue curve of the universal modeling (orange curve) used in LIM and the task-specific modeling (blue curve) used in traditional quantitative investment research, for 7 commodity futures: RU, PB, B, SP, P, FB, PP and for 2 stock index futures IF and IH. }
        \label{futures_backtest_netvalue}
    \vspace{-10pt}
\end{figure*}

Table~\ref{tab:comparison_stocks_futures} and Figure~\ref{futures_backtest_netvalue} present the experimental results comparing universal modeling with task-specific modeling across various futures instruments. The results indicate that, for the majority of futures instruments, the universal modeling approach outperforms the task-specific models in several key metrics, including annual return, Sharpe ratio, maximal drawdown, and Information Coefficient (IC). Notably, the net value curves associated with the universal models are generally much smoother and more stable compared to those of the task-specific models, as evidenced by the significantly straighter trajectory of the universal model curves. 

This stability suggests that the universal model is more resilient to market fluctuations, thereby offering a more consistent performance over time. Even in cases where the universal model's returns for instruments such as P, FB, and IH do not exceed those achieved by the task-specific models, the Sharpe ratio of the universal model is markedly higher. This indicates that the universal model delivers superior risk-adjusted returns, outperforming task-specific models in managing volatility and preserving capital. The enhanced Sharpe ratio highlights the universal model's ability to achieve a more favorable balance between return and risk, even when raw returns are not always higher. These findings underscore the robustness and efficiency of universal modeling in a diverse range of trading environments, demonstrating its potential as a more effective approach for futures trading strategies.
